# Supplementary material for: Differentiable Stripe Patterns for Inverse Design of Structured Surfaces
Source: arXiv:2305.13841 source file (2023-05-23)
Supplement: Supplementary file 1 [file Appendix.tex]

\appendix

\section{IPC rod-rod distance derivatives}
distance barrier item for rods:

\begin{equation}
    b(\dprime,\dhat) = -(\dprime-\dhat)^2 \ln(\frac{\dprime}{\dhat})
\end{equation}
\begin{equation}
    \dprime = (\sqrt{d}-g)^2
\end{equation}
where $d$ is a squared distance between two primitives, and $\dprime$ is the squared distance between two rods, $g$ is the smallest gap between two primitives, e.g., $g=2r$. Rewriting the above equations, we have
\begin{equation}
    b(d,\dhat) = -((\sqrt{d}-g)^2-\dhat)^2 \ln(\frac{(\sqrt{d}-g)^2}{\dhat})
    \label{eq:rodDistanceBarrier}
\end{equation}

First-order derivative $\frac{db}{dd} = \frac{db}{d\dprime}\frac{d\dprime}{dd}$, where corresponding first-order derivatives are
\begin{equation}
    \frac{d b}{d \dprime} = -2(\dprime - \dhat)\ln(\frac{\dprime}{\dhat})-(\dprime-\dhat)^2\frac{1}{\dprime} \ ,
\end{equation}
\begin{equation}
    \frac{d\dprime}{dd} = 1-\frac{g}{\sqrt{d}}
\end{equation}
Then, we can compute $\frac{db}{dx} = \frac{db}{dd}\frac{dd}{dx}$.

Second-order derivative $\frac{d^2b}{dd^2} = \frac{d^2b}{d\dprime^2}(\frac{d\dprime}{dd})^2 + \frac{db}{d\dprime}\frac{d^2\dprime}{dd^2}$, where corresponding second-order derivatives are
\begin{equation}
    \frac{d^2b}{d\dprime^2}=-2\ln(\frac{\dprime}{\dhat})-4(\dprime-\dhat)\frac{1}{\dprime}+(\dprime-\dhat)^2\frac{1}{\dprime^2} \ ,
\end{equation}
\begin{equation}
    \frac{d^2\dprime}{dd^2}=\frac{g}{2}d^{-3/2}
\end{equation}

\section{derivatives for parallel edges}
Due to transformation of periodic boundary conditions, the derivatives for parallel edges also need to be updated as following:
For parallel edges, their barrier energy is $\kappa e_k(\bx)b(d_k(\bx))$. Its gradient with respect to $\bx_a$ is
\begin{equation}
    \frac{d \kappa e_k(\bx)b(d_k(\bx))}{d \bx_a} = \kappa b(d_k(\bx))\frac{d e_k(\bx)}{d \bx}^T\frac{d\bx}{d\bx_a} + \kappa e_k(\bx)\frac{d b}{d d}\frac{d d}{d \bx}^T\frac{d\bx}{d\bx_a}
\end{equation}
and its hessian is
\begin{multline}
    d(\frac{d \kappa e_k(\bx)b(d_k(\bx))}{d \bx_a})/d\bx_a = \kappa (\frac{d e_k(\bx)}{d\bx}^T\frac{d\bx}{d\bx_a})^T \frac{d b}{d d}\frac{d d}{d \bx}^T\frac{d\bx}{d\bx_a} \\
    + \kappa b(d_k(\bx))(\frac{d\bx}{d\bx_a}^T\frac{d^2 e_k(\bx)}{d\bx^2}\frac{d\bx}{d\bx_a} + \frac{d e_k(\bx)}{d\bx}^T\frac{d^2\bx}{d\bx_a^2}) \\
    + \kappa (\frac{d b}{d d}\frac{d d}{d \bx}^T\frac{d\bx}{d\bx_a})^T \frac{d e_k(\bx)}{d\bx}^T\frac{d\bx}{d\bx_a}\\
    + \kappa e_k(\bx)\left((\frac{dd}{d\bx}^T\frac{d\bx}{d\bx_a})^T\frac{d^2b}{dd^2}\frac{dd}{d\bx}^T\frac{d\bx}{d\bx_a} + \frac{db}{dd}(\frac{d\bx}{d\bx_a}^T\frac{d^2d}{d\bx^2}\frac{d\bx}{d\bx_a}+\frac{dd}{d\bx}^T\frac{d^2\bx}{d\bx_a^2})\right)
\end{multline}

\section{adaptive barrier stiffness}
If $\kappa$ is not set appropriately, the contact primitives would either need to get extremely close to get enough repulsion (barrier gradient) when $\kappa$ is too small, or need to get a distance right below $\hat{d}$ for a small repulsion if $\kappa$ is set too
large, both resulting in slow convergence because of ill-conditioning and nonsmoothness. Thus adaptively setting and/or adjusting $\kappa$ is essential.

Tiny distances not only make CCD less robust and make the optimization less efficient in our numerical simulation, but also are not physically reasonable in science.

the convergence problem is caused by the upper bound of the adaptive stiffness of the contact force. After setting a larger value the convergence problem has been addressed.
However, a larger value of stiffness will induce numerical float precision problem, which makes the convergence bad after certain gradient value, e.g., 1e-16.
If the above numerical problem occurs, we treat is as converge when the gradient norm smaller than a threshold and gradient difference between two successive gradient smaller than 1e-20.

\section{Elliptical cross section}
For an elliptical cross section edge with two ends $\be_0$ and $\be_1$ and the edge rotation $\theta_e$, the surface point $\bp_e$ can be determined by 
\begin{equation}
    \bp_e = l \be_0 + (1-l) \be_1 + \cos(\phi_{e2})r_1 \mathbf{f}_1 + \sin(\phi_{e2})r_2 \mathbf{f}_2 \ ,
\end{equation}
where $\bt = \be_0 - \be_1$, $\mathbf{f}_1$ and $\mathbf{f}_2$ are orthogonal frames. Since we need to find  the contact point within the edge, $l$ should satisfy $l\in[0,1]$. So we further parameterize $l=(1+\tanh(\phi_{e1}))/2$ instead of solving a constrained problem. We aggregate parameters as $\boldsymbol{\phi_e} =\left[\phi_{e1}, \phi_{e2}\right]$, so the gradient and hessian of the surface point with respect to $\phi_e$ are, respectively,
\begin{equation}
    \frac{d \bp_e}{d \boldsymbol{\phi_e}} = 
    \begin{bmatrix}
    \frac{1}{2}(\be_0-\be_1)(1-\tanh^2(\phi_{e1})) &
    -\sin(\phi_{e2})r_1\mathbf{f}_1 + \cos(\phi_{e2})r_2\mathbf{f}_2
    \end{bmatrix} \ ,
\end{equation}
\begin{equation}
\begin{split}
    \frac{d^2 \bp_e}{d \boldsymbol{\phi_e}^2} & =
    \begin{bmatrix}
    \mathbf{0} & -(\be_0-\be_1)\tanh(\phi_{e1})(1-\tanh^2(\phi_{e1}))
    \end{bmatrix}\\
    & \quad
    \begin{bmatrix}
     -\cos(\phi_{e2})r_1\mathbf{f}_1 - \sin(\phi_{e2})r_2\mathbf{f}_2 & \mathbf{0}
    \end{bmatrix}
\end{split} \ .
\end{equation}
In addition, for the computation of IPC contact, we also need to compute surface point gradient and hessian with respect to $\bx_e = [\be_0, \be_1, \theta_e]$, so we have
\begin{equation}
\frac{d \bp_e}{d \bx_e} = \frac{\partial \bp_e}{\partial \boldsymbol{\phi_e}}\frac{d \boldsymbol{\phi_e}}{d \bx_e} + \frac{\partial \bp_e}{\partial \bx_e}
\end{equation}
where $\frac{\partial \bp_e}{\partial \bx_e}$ is easy to compute. Note that the orthogonal frames are also determined by $\bx_e$. Whereas $\frac{d \boldsymbol{\phi_e}}{d \bx_e}$ needs to solve a linear system for a given constraint, we will revisit this gradient later.

For vertex related contact we place an ellipsoid at the vertex $\bv$, the surface point $\bp_v$ can be determined by
\begin{equation}
    \bp_v = r_1 \cos(\phi_{v0}) \cos(\phi_{v2}) \bt +  r_1 \cos(\phi_{v0})\sin(\phi_{v2}) \mathbf{f}_1 + r_2 \sin(\phi_{v0}) \mathbf{f}_2
\end{equation}
where $\bt$, $\mathbf{f}_1$ and $\mathbf{f}_2$ are frames determined by its connected edges. Since $\phi_{v1}\in[-\frac{\pi}{2},\frac{\pi}{2}]$, we also parameterize it as $\phi_{v0}=\frac{\pi}{2}\tanh(\phi_{v1})$. Similar to the edge situation, we also aggregate parameters as $\boldsymbol{\phi_v} = \left[\phi_{v1},\phi_{v2}\right]$. So the gradient of the surface point with respect to $\phi_v$ is
\begin{equation}
    \frac{d \bp_v}{d \boldsymbol{\phi_v}} = 
    \begin{bmatrix}
    \scriptscriptstyle (-r_1\sin(\phi_{v0})\cos(\phi_{v2})\bt - r_1\sin(\phi_{v0})\sin(\phi_{v2}) \mathbf{f}_1 + r_2 \cos(\phi_{v0})\mathbf{f}_2) \frac{\pi}{2}(1-\tanh^2(\phi_{v1})) \\
    -r_1 \cos(\phi_{v0}) \sin(\phi_{v2}) \bt +  r_1 \cos(\phi_{v0})\cos(\phi_{v2}) \mathbf{f}_1
    \end{bmatrix}^T \ ,
\end{equation}
and hessian $\frac{d^2 \bp_v}{d \boldsymbol{\phi_v}^2}$ can also be computed similarly.

\subsection{Minimum distance between primitives}
 To compute contact pair between two primitives, we need to compute minimum distance between them. However, there is no closed form to compute minimum distance between two elliptical primitives. So we compute minimum distance between them by
\begin{equation}
    \argmin_{\boldsymbol{\phi_+}, \boldsymbol{\phi_*}}  \quad d=\|\bp_+(\boldsymbol{\phi_+}) - \bp_*(\boldsymbol{\phi_*})\|^2
\end{equation}
where $\bp_+$ and $\bp*$ are two surface points on an ellipsoid or an elliptical cross section edge and $\boldsymbol{\phi_+}$ and $\boldsymbol{\phi_*}$ are their corresponding parameters, respectively.

After finding the minimum point, we need to compute gradient and hessian, respectively,
\begin{equation}
    \frac{dd}{d\bx_+} = \frac{\partial d}{\partial \bp_+}\frac{\partial \bp_+}{\partial \bx_+} = \frac{\partial d}{\partial \bp_+}\left( \frac{\partial \bp_+}{\partial \boldsymbol{\phi_+}}\frac{d \boldsymbol{\phi_+}}{d \bx_+} + \frac{\partial \bp_+}{\partial \bx_+}\right) \ ,
\end{equation}
\begin{multline}
    \frac{d^2d}{d{\bx_+}^2} = \left( \frac{\partial \bp_+}{\partial \boldsymbol{\phi_+}}\frac{d \boldsymbol{\phi_+}}{d \bx_+} + \frac{\partial \bp_+}{\partial \bx_+}\right)^T \frac{\partial^2 d}{\partial {\bp_+}^2}\left( \frac{\partial \bp_+}{\partial \boldsymbol{\phi_+}}\frac{d \boldsymbol{\phi_+}}{d \bx_+} + \frac{\partial \bp_+}{\partial \bx_+}\right)\\
    + \frac{\partial d}{\partial \bp_+}\left( \left(\frac{\partial \phi_+)}{\partial \bx_+}\right)^T
    \left(\frac{\partial^2 \bp_+}{\partial {\phi_+}^2}\frac{\partial\phi_+}{\partial\bx_+}+\frac{\partial^2 \bp_+}{\partial\phi_+\partial\bx_+}\right) + \frac{\partial\bp_+}{\partial\phi_+}\frac{d^2\phi_+}{d{\bx_+}^2} + \frac{\partial \bp_+}{\partial \bx_+ \partial\phi_+}\frac{\partial\phi_+}{\partial\bx_+} + \frac{\partial^2\bp_+}{\partial{\bx_+}^2}
    \right)
\end{multline}
for optimizing IPC. Note that the gradient $\frac{dd}{d\bx_*}$ and hessian $\frac{d^2d}{d{\bx_*}^2}$ can also be computed in similar way.

To compute these derivatives, we base on the minimum distance gradient $\frac{d d}{d [\boldsymbol{\phi_+},\boldsymbol{\phi_*}]}=\mathbf{0}$ which give us two constraints $\frac{d d}{d \boldsymbol{\phi_+}}=0$ and $\frac{d d}{d \boldsymbol{\phi_*}}=0$ due to independency between $\boldsymbol{\phi_+}$ and $\boldsymbol{\phi_*}$. So we can use these two constraints to compute the gradients $\frac{d \boldsymbol{\phi_+}}{d \bx_+}$ and $\frac{d \boldsymbol{\phi_*}}{d \bx_*}$, respectively. Based on this, starting from the constraint
\begin{equation}
    \frac{d d}{d \boldsymbol{\phi_+}} = \frac{d d}{d \bp_{+}}\frac{d \bp_+}{d \boldsymbol{\phi_+}} = 0
\end{equation}
and taking the derivative with respect to $\bx_+$, we have
\begin{equation}
\label{MinDistanceFirstOrderSensitivityAnlysis}
    \left(\frac{\partial \bp_+}{\partial \phi_+}\right)^T \frac{\partial^2d}{\partial{\bp_+}^2} \left(\frac{\partial \bp_+}{\partial \phi_+}\frac{d\phi_+}{d \bx_+} + \frac{\partial \bp_+}{\partial \bx_+} \right) + 
    \frac{\partial d}{\partial \bp_+}\left(\frac{\partial^2\bp_+}{\partial {\phi_+}^2}\frac{d\phi_+}{d\bx_+} + \frac{\partial^2\bp_+}{\partial \phi_+\partial \bx_+}\right)= \mathbf{0} \ .
\end{equation}
After reformulating the above equation, the above equation yields
\begin{equation}
\textstyle
    \left(\left(\frac{\partial \bp_+}{\partial \phi_+}\right)^T \frac{\partial^2d}{\partial{\bp_+}^2}\frac{\partial \bp_+}{\partial \phi_+} +
    \frac{\partial d}{\partial \bp_+}\frac{\partial^2\bp_+}{\partial {\phi_+}^2}
    \right)
    \frac{d\phi_+}{d\bx_+}
    = -\left(\frac{\partial \bp_+}{\partial \phi_+}\right)^T \frac{\partial^2d}{\partial{\bp_+}^2}\frac{\partial\bp_+}{\partial\bx_+} -\frac{\partial d}{\partial \bp_+}\frac{\partial^2\bp_+}{\partial \phi_+\partial \bx_+} \ .
\end{equation}
Therefore, we can solve this linear system to obtain $\frac{d\phi_+}{d\bx_+}$. By using the same fashion, we can also get $\frac{d\phi_*}{d\bx_*}$. To obtain $\frac{d^2\phi_+}{d{\bx_+}^2}$, we further take the derivative of Eq.\ref{MinDistanceFirstOrderSensitivityAnlysis} with respect to $\bx_+$ and obtain

\begin{multline}
   \left(\frac{\partial^2d}{\partial{\bp_+}^2} \left(\frac{\partial \bp_+}{\partial \phi_+}\frac{d\phi_+}{d \bx_+} + \frac{\partial \bp_+}{\partial \bx_+} \right)\right)^T \frac{\partial^2\bp_+}{\partial{\phi_+}^2} \left(\frac{\partial^2d}{\partial{\bp_+}^2} \left(\frac{\partial \bp_+}{\partial \phi_+}\frac{d\phi_+}{d \bx_+} + \frac{\partial \bp_+}{\partial \bx_+} \right)\right) \\
   + \left(\frac{\partial \bp_+}{\partial \phi_+}\right)^T \left(\frac{\partial \bp_+}{\partial \phi_+}\frac{d\phi_+}{d \bx_+} + \frac{\partial \bp_+}{\partial \bx_+} \right) \notate{\frac{d^3\bp_+}{d{\bp_+}^3}}{1}{=0} \left(\frac{\partial \bp_+}{\partial \phi_+}\frac{d\phi_+}{d \bx_+} + \frac{\partial \bp_+}{\partial \bx_+} \right) \\
   \textstyle
   + \left(\frac{\partial \bp_+}{\partial \phi_+}\right)^T \frac{\partial^2 d}{\partial{\bp_+}^2} \left(\left(\frac{\partial\phi_+}{\partial\bx_+}\right)^T\left(\frac{\partial^2\bp_+}{\partial{\phi_+}^2}\frac{\partial\phi_+}{\partial\bx_+}+\frac{\partial\bp_+}{\partial\bx_+}\right) + \frac{\partial\bp_+}{\partial\phi_+}\notate{\frac{d^2\phi_+}{d{\bx_+}^2}}{1}{}+\frac{\partial^2\bp_+}{\partial{\bx_+}^2}+\frac{\partial^2\bp_+}{\partial\bx\partial\phi_+}\frac{\partial\phi_+}{\partial\bx_+}\right) \\
   + \left(\frac{\partial^2\bp_+}{\partial {\phi_+}^2}\frac{d\phi_+}{d\bx_+} + \frac{\partial^2\bp_+}{\partial \phi_+\partial \bx_+}\right)^T \frac{\partial^2 d}{\partial{\bp_+}^2} \left(\frac{\partial^2\bp_+}{\partial {\phi_+}^2}\frac{d\phi_+}{d\bx_+} + \frac{\partial^2\bp_+}{\partial \phi_+\partial \bx_+}\right)\\
   \textstyle
   + \frac{\partial d}{\partial \bp_+}\left( \left( \frac{d\phi_+}{d\bx_+}\right)^T\left(\frac{\partial^3\bp_+}{\partial{\phi_+}^3}\frac{d\phi_+}{d\bx_+}+\frac{\partial^3\bp_+}{\partial{\phi_+}^2\partial\bx_+}\right)+\frac{\partial^2\bp_+}{\partial{\phi_+}^2} \notate{\frac{d^2\phi_+}{d{\bx_+}^2}}{1}{} +\frac{\partial^3\bp_+}{\partial\partial\phi_+\partial\bx_+\partial\phi_+}\frac{d\phi_+}{d\bx_+}+
   \notate{\frac{\partial^3\bp_+}{\partial\phi_+\partial{\bx_+}^2}}{1}{=0}
   \right)
   \\ = \mathbf{0}
\end{multline}

\section{Periodicity with midsurface}

With the midsurface $\varphi$, we enforce periodicity of rod structures for one side of edge $e0$ and opposite side edge $e1$, where edge $e0$ has direction from vertex $x0$ to vertex $x1_{eq}$ with $x1_{eq}$ as boundary vertex, and edge $e1$ has direction from vertex $x1$ to vertex $x2$ with $x1$ as equivalent boundary vertex to $x1_{eq}$. Therefore, to enforce periodicity between these two connected boundary edges, we first use rest configuration as parametric coordinate $X0_{tr} = X0+(X1-X1_{eq})$. We, then, use the midsurface to get its transformed position $x0_{tr}=\varphi(X0_{tr})+h\bn(x0_{tr})+R(x0_{tr})R(x0)^T\Tilde{\bu(x0)}$. Finally, we use $x0_{tr}$, $x1$ and $x2$ to compute energies of bending and twist.

For rigid-body and rod connection, we will first multiply the rotation matrix $\bR_{\varphi}$ getting from midsurface to compute the deformed frame at local state. Then, we will multiply accumulated rotation matrix $\bR_{a}$ and delta rotation matrix $\bR_{d}$ to avoid gimbal lock.

\subsection{Transformation of periodic boundary conditions}

Since each virtual vertex $\bx_v$ is computed by its real vertex $\bx_r$ in the unit cell and the planar transformations $\bd_{ij}$ and $\bd_{kl}$, where $\bd_{ij} = \bx_j - \bx_i$ and $\bd_{kl} = \bx_l - \bx_k$ are computed by using their corresponding two reference real vertices, respectively, as shown in Fig. \ref{fig:periodicBoundaryConditions}. The position of the virtual vertex, therefore, can be determined by a transformation function $\bx_v = \bT(\bx_{map})$, where $\bx_{map} = [\bx_r, \bx_j,\bx_i, \bx_l,\bx_k]$.

For the computation of a scalar function $d(\bx)$, e.g., distance functions and energy functions, with $n$ vertices $\bx = [\bx_1,\dots,\bx_i,\dots,\bx_n]$, we need to compute its gradient and hessian when applying optimization. The positions of virtual vertices depend on real vertices, so the scalar function actually depends on $\bx_a = {[\bx_{r1},\dots,\bx_{ri},\dots,\bx_{rn}},\\ \bx_j, \bx_i, \bx_l, \bx_k]$, where $\bx_{ri} = \bx_{i}$ if $\bx_{i}$ is a real vertex, otherwise it is the corresponding real vertex $\bx_r$ of the virtual vertex $\bx_i$. The vertices $\bx_j, \bx_i, \bx_l, \bx_k$ are reference vertices for the periodic boundary conditions use for the transformation of all virtual vertices. The gradient of the scalar function $d$ with respect to $\bx_a$ is 
\begin{equation}
    \bG = \frac{d d(\bx)}{d\bx}^T\frac{d\bx}{d\bx_a} \ ,
\end{equation}
and its hessian is
\begin{equation}
    \bH = d(\frac{d d(\bx)}{d\bx}^T\frac{d\bx}{d\bx_a}) / d\bx_a = (\frac{d\bx}{d\bx_a})^T\frac{d^2 d(\bx)}{d\bx^2}\frac{d\bx}{d\bx_a} + \frac{d d(\bx)}{d\bx}^T\frac{d^2\bx}{d\bx_a^2}
\end{equation}
where $\frac{d d(\bx)}{d\bx}^T\frac{d^2\bx}{d\bx_a^2} = 0$ if $\bT$ is a linear transformation, i.e., planar periodic boundary conditions.
